# Supplementary material for: Confidential Attestation: Efficient in-Enclave Verification of Privacy Policy Compliance
Source: arXiv:2007.10513 source file (2020-07-20)
Supplement: Supplementary file 1 [file Appendix_last_time_review.tex]

% \onecolumn
\section*{Reviews and Summary of Revision}

\noindent Following are the reviews we received from our latest submission to IEEE S\&P 2020, and our summary of changes following the reviews.

\section{Summary of revision}
Following the reviews from IEEE S\&P 2020, we have made the following major improvements to this paper.

\vspace{3pt}\noindent\textbf{Better highlighted the novelty}.
We elaborated the strengths of our work (Section~\ref{sec-introduction}) and compared them with the most related works (Section~\ref{sec-relatedwork}). To the best of our knowledge, we are the first one proposing the CAT model and trying to address the confidential attestation dilemma (that the service code provider is reluctant to expose the implementation details of its services for public attestation) with the unbalanced proof carrying code framework. Barely related work takes into account the privacy issues of both code providers and data owners. Works such as Ekiden~\cite{cheng2018ekiden} provide a computing environment for running a smart contract on sensitive data privately. However, they only care about the confidentiality of the input data and the contract state, but don't need to cope with the secrecy of contract(program) because of its transparency. Thus, the CAT model solves a disparate problem in a totally different scenario.

Fortunately, the confidential attestation challenge can be addressed perfectly using Proof Carrying Code (PCC) framework.
According to the XFI~\cite{erlingsson2006xfi}, a brilliant work co-authored by the designer -  George C. Necula, XFI modules can be seen as an example of proof-carrying code, even though they do not include logical proofs. Similar as XFI, our work uses static analysis with inline software guards that perform checks at runtime, which could be regarded as an example of PCC that trusts only the verifier, not the means of proof generation.

Sand-boxing is a suitable technique to perform privacy-preserving computations. Related works like Ryoan~\cite{hunt2018ryoan} leverage Google NaCl to build its prototype, whose core library is about 19 MB including several LLVM components. Instead, our implementation is more lightweight, adding about 2MB of binary code to the TCB.

On the other side, our approach is more practical compared with formal methods, e.g., a type-safe language. A type-safe language compiler/interpreter along cannot finish the verification of properties such as confidentiality.  A verification condition generator (VCGen) and a proof solver should work together with the compiler/interpreter, which introduce huge TCB and computation overhead.
In our design, we let the proof generator (the customized LLVM) to provide rich control/data flow information and then check them strictly inside the enclave, which removes the compiler from the TCB and further helps saving memory consumption and performance overhead. And we fully considered the characteristics of policy-compliant computations before proposing our design. Real-world applications often contain hundreds of lines of code, and thousands of instructions. Comparing to formal verification, generating security annotations is significantly less weighted, allowing our solution to scale to real world software of such amount of code.

\vspace{3pt}\noindent\textbf{Added more policies}. We extended the number of policies that we need to enforce from 5 to 7, to fully protect the privacy of user data. These policies include data leak control, control-transfer management, self-modifying code block, and side/covert channel mitigation. We used the implemented prototype to demonstrate how policies can be enforced (using an unbalanced design of assembly level instrumentations on the code provider side with a lightweight verification on the code consumer side). 

Those additional policies including input/output constraint (P0) and side/covert channel mitigation (P6) are described (Section~\ref{subsec-policies}), which are designed to limit the amount of information an attacker can get. Specifically, attackers can not access the plaintext of input/output message directly via enforcing P0. We made OCall stubs for calling system calls. Restrictions on the length of OCall stubs can handle the issue of the Intel SGX SDK's Null-terminated string.
Enforcing P6 could protect the data owner from page fault-based controlled channel attacks and most L1/L2 cache-based side channel attacks. 
Meanwhile, Data Execution Prevention (DEP) can not be skipped since the loaded binary will be allocated on enclave's heap memory, leading to a W+X problem. The goal of enforcing DEP (P4) was elaborated in Section~\ref{subsec-policies}. This will not be a problem in SGXv2 since dynamic memory management of EPC is introduced in the new version of SGX hardware, which can protect dynamic loaded pages with permission changing and verifying instructions such as \texttt{EAUG/EMODPE/EACCEPT}.

\vspace{3pt}\noindent\textbf{Enriched implementation details}.
We added details on how the proof is generated and how the whole system works (Section~\ref{sec-implementation} and Appendix~\ref{appendix-instrumentation}). Specifically, we illustrate how to use CAT to implement information release prevention policies and common SGX side/covert channel alleviation policies. 

We built an assembly-level PCC framework from scratch. The instrumentation module for enforcing P1 and also be used in enforcing DEP, aka. P4, with few modification.
We showed that the code generator consists of portable components, which introduces a great flexibility for supporting replaceable policies. Wider policies can be integrated via implementing other LLVM passes.

Exquisite implementation was applied in building one bootstrap enclave as well (Section~\ref{subsec:bootstrap-impl}). We illustrated how the loader and the verifier can be integrated seamlessly (Section~\ref{subsec-loading}). The binary parsing module in the loader (in Figure~\ref{fg-workflow}) is  not only designed for assisting to get offsets for relocation, but also can give the program entry for later disassembling. Moreover, legal indirect branch labels need to be translated by the binary parser. The loader and the verifier formed a whole and work in harmony.

Our implementation did not use two enclave for separating the verification stage and the code loading and execution stage. The only advantage of using two enclaves is that there will be no W+X issue during the target binary loading, which actually can be dealt with the software DEP. Meanwhile, using two enclave may induce more communication overhead. The attestation protocol should be re-designed, while introduces larger TCB and more overhead since more parties are involved.
%More importantly, if we consider it more carefully, it still needs a binary rewriter within the one bootstrap enclave. 

We believe both designs are reasonable. However, at this time, we may stick to the original ``one-enclave'' design for the following reasons. Firstly, memory store operation instrumentation can be easily extended to support W+X. Secondly, within the one-enclave design, the code of resolving symbols (during loading) can be easily reused by the rewritter and the verifier which reduces the memory consumption of limited enclave memory. 
%One-enclave design is more compact and cute, which leads a smaller TCB.

\vspace{3pt}\noindent\textbf{Thoroughly evaluated the CAT system}.
We built more benchmarks (including micro-benchmarks and real-world applications) and tested them with the prototype we implemented (Section~\ref{subsec-experiments}). Performance analysis was given, showing the difference under multiple granularities of protections (P1, P1+P2, P1\textasciitilde P5, and P1\textasciitilde P6). Security suggestions on which policies should be incorporated can be made according to their performance and what security properties they can bring in at different scenarios.

In addition, the TCB of our CAT system was evaluated. Policies had been analyzed for soundness and completeness as well (Section~\ref{subsec-securityanalysis}). 
The goal of enforcing policies on memory write operations is to build an information confinement, and a CFI policy can gruarantee the check on other policies cannot be circumvented.

\vspace{3pt}\noindent\textbf{Better summarized the lessons learnt}.
We have to acknowledge that our current CAT-SGX system has limitations and we discussed them in Section~\ref{sec-discussion}. We summarized those limitations as follows.

Side channels have been recognized as a major threat for SGX. Attacks include cache, TLB, branch prediction, page table, etc. Side channel defenses for SGX remains an important research problem. 
%To the best of our knowledge, ours is the first work showing how to support side channel defenses verification by flexible security policy enforcement.
With the help of SSA monitoring to detect and prevent AEX-based channels, our work can limit the data leakage via most interrupt-based covert channels. Further, covert channel based on parameters of system calls can be eliminated by enforcing P0 - a strong constraint on input/output messages that only allows certain syscalls (\texttt{send/recv}). System functions like setjmp/longjmp are disallowed in our system since they can break
call-return semantics.
System call interval can not be a covert channel in CDaaS cases since we only process input/output once during the in-enclave service. Individual request can only leak few bits. However, it can be a threat in CCaaS scenarios such as web-server as a service. Attackers can deliberately construct requests which would cost different processing time, and transfer some secrets via the processing time difference. Overall, we have to admit that our work cannot take over all kinds side/covert channels, policies to defend against them (e.g., fixed processing time) can be added into our framework though.

Multi-threading/Multi-user is not supported currently, but can be accomplished with certain extensions. We elaborated how our work can be extended towards solving those issues in Section~\ref{sec-discussion}. Supporting the single-thread multi-user scenario could be very easy by adding a data cleansing policy as well as a session key management for multiple users. Unfortunately, supporting a multi-thread scenario would take much more effort. 
Recent works have been proposed on this hot topic. Occlum~\cite{shen2020occlum} and MPTEE~\cite{zhao2020mptee} both leverage Intel MPX~\cite{shen2018isolate} to isolate the address space between multiple threads for multitasking efficiently. Although, incluing LibOS into the TCB may not be accepted, we can learn from them and  memory read auditing policies for reserved regions for different threads. Specifically, the code provider can divide the `.data' section of the target program into memory spaces for $N$ threads.
Then on the bootstrap enclave side, the loader should keep the upper/lower bounds when performing thread switch, and the verifier can enforce the memory accessing policies for all $N$ threads.

%%%%%%%%%%%%%%%%%%%%%%%%%%%%%%%%%%%%%%%%%%%%%%%%%%%%%
%reviews

\section{Reviews}

\begin{markdown}
## Review A
=================================================

### Brief Paper Summary  

The paper proposes CAT, an approach for ensuring to a user that code meets privacy requirements without the user observing the code.  CAT relies on a combination of compiler modification to generate code that meets the privacy requirements and an SGX enclave that loads and execute the code only after verifying it meets the requirements.

### Strengths

Ensuring data privacy is important.

### Weaknesses

There is a huge gap between what the paper promises and what it delivers
Considering what is being delivered, it's not clear what the novelty is.

### Detailed Comments for Authors

Thank you for submitting your work to IEEE SP.  While I appreciate the amount of work that went into CAT, I am afraid that I cannot recommend that the work be accepted.

The paper starts with a promise of a framework that can validate the compliance of code with privacy policies. However, it only investigates a single privacy policy. There is absolutely no discussion of how the research can be extended to other privacy policies, and such extensions do not seem trivial.

The privacy policy the paper claims to enforce is to ensure that data is not leaked from the enclave.  The paper reduces this policy to five requirements (P1-P5, Page 6).  While I agree that all requirements are necessary for enforcing the policy, I am not convinced that they are sufficient.  In particular, I do not see that these requirements are sufficient to prevent data from one query leaking into another.  In the case of a service provider that provides a service to multiple clients, this would allow leaking information between clients.  Another potential information leak is via system calls or their arguments - the paper indicates that system calls are supported but does not explain how their arguments are validated.

When reducing the problem to only maintaining the five requirements, it is not clear what the advantage of the suggested approach over using type-safe languages or mechanisms such as suggested for Google Chrome Native Clients (Yee et al. IEEE SP 2009).

Side channel attacks are considered out-of-scope for the paper. However, given the vulnerability of SGX to such attacks, and the attempt to protect from malicious code, ignoring these seem to render CAT completely useless for protecting privacy.

There is absolutely no discussion of the limitations of the approach. Can the verified code communicate with the service provider? Can it use longjmp? Is multithreading supported? etc.

Overall, I think that the idea is promising, but the gap between the promise and the current implementation is too wide.  I suggest that the authors work on reducing the gap e.g. by showing how the approach could apply for a wider range of security/privacy policies.

## Review B
=================================================

### Brief Paper Summary

This paper proposes to solve a problem with remote attestation as used in SGX. One party provides code and another provides data; neither wants to provide their part in the clear; but the party providing data needs to be sure that their data's privacy is assured.  They propose to do this with a loader enclave that checks and runs proof-carrying code (PCC) guaranteed to comply with the privacy policy.

### Strengths

The system is relatively simple.

### Weaknesses

The simplicity of this system comes from its lack of expressiveness, and fixed not-very-useful security policy.

The lack of covert channel protection is very problematic.  There's not much point in blocking the front door if the back door is wide open.  While unintentional side channels can be tricky to exploit, covert channels are really easy.

The only supported policy is that no data is written outside the enclave.  It is not clear how the loader will determine whether the results of the computation comply with any kind of privacy policy, which is implied in some of the suggested use cases.  In fact, the paper doesn't discuss how output is to be produced at all, though I assume that the loader would have a trusted output routine of some kind.

The paper is riddled with typos.

This isn't proof-carrying code.  It's instrumented code.

I'm not clear why this would be better in practice than a LISP interpreter with some security/privacy policy annotations.  If you must run binary code, why must the loader be in the same enclave as the running code?  Surely verifying it from afar would be safer and would avoid some of this CFI mess?

### Detailed Comments for Authors

needs certified -> needs to be certified

quite larger -> significantly larger

unintended redirected -> redirected,

conclude with malicious OS or hypervisor -> collude with a malicious OS or hypervisor

during the compiling -> during compilation

would leakage user's data -> would leak users' data
rewritting -> rewriting

As mentioned above, to facilitate PCC framework working well -> cut this paragraph, you said it already

Instrumentations -> Instrumentation

Theses -> These

stack pointer never point -> stack pointer never points

cannot modify alter -> cannot modify

i.e., one does not use external elements -> i.e., one that does not use external elements

code generator firstly extract -> code generator first extracts

is very small that only consists -> consists

500 lines that is made from scratch -> 500 new lines of code (in addition to ...).

more small and exquisite -> smaller and more exquisite

but leverage -> but leverages

we still want to acclaim -> we still claim [or expect?]

## Review C
=================================================

### Brief Paper Summary

The paper makes three main contributions: the CAT model where the privacy of
both code and data are preserved (leakage is limited to what the code/data
premptively agree to), a proof-carrying code based implementation to reduce
the trusted code base size (TCB), and performance/programmability evaluation.

### Strengths

The paper includes a pragmatic set of decisions to reduce the TCB
of a two-way (between data owner and code owner) privacy contract.

### Weaknesses

The CAT model has been proposed and studied extensively; often coupled
with a blockchain based audit logs of the transaction between the code-
and data-owner.

Examples: 

- private data objects (Intel): https://arxiv.org/abs/1807.05686

- similar paper (cheng et al): https://arxiv.org/abs/1804.05141

and others.

The advance of CAP over a standard attestation protocol is a direct
extension -- perhaps I am missing something.

### Detailed Comments for Authors

Good work! I like the problem space -- this is in an area where advances can be very impactful towards building a low TCB system where data-owners and code-owners can transact.

The paper can be greatly improved by focusing and going deeper into what is new here.

The attestation protocol might be new; but I couldn't figure out why. 
Allocating the tasks across untrusted and trusted parts, with one generating the proof while a simpler trusted part checks it inside the enclave seems novel and worth leading the story with. Bolting on DEP etc protections to cover for SGX v1 details seems unnecessary -- can this be skipped?

If focusing on the second theme above, it would be great to discuss the
properties and their impact on proof gen/verification.

Security properties that are being checked: (leaving out DEP etc)
- prevent explicit stores of data outside the enclave range
- prevent implicit spills out of the enclave
- prevent tampering of the bootstrap enclave contents

Should these be enforced in hardware (if the goal is to use hardware-based enclaves like SGX)? Why should this require a proof-carrying code -- I am not sure and would love to learn more.

Interestingly, I can see why one might want to verify side-channel security of code that runs inside an enclave and ensuring that side-channel defenses compiled into the code indeed check off certain properties.

Overall, I am very supportive of this problem and the effort seems honest -- I couldn't pinpoint the key advances that this paper really pushes, but am happy to be convinced otherwise.

\end{markdown}

%%%%%%%%%%%%%%%%%%%%%%%%%%%%%%%%%%%%%%%%%%%%%%%%%%%%%%%%%%%

\ignore{

\section{Response to reviews}

To Review A:

Comment 1. *”...There is absolutely no discussion of how the research can be extended to other privacy policies, and such extensions do not seem trivial...The privacy policy the paper claims...While I agree that all requirements are necessary for enforcing the policy, I am not convinced that they are sufficient...”*

We extend the number of policies that we need to enforce from 5 to 9, to fully protect the privacy of user data. Proofs are sufficient, which were proved in previous work.

Comment 2. *”Another potential information leak is via system calls or their arguments - the paper indicates that system calls are supported but does not explain how their arguments are validated”*

We made Ocall stubs for calling system call. Restrictions on all Ocall stubs output length, including string type of parameters, can handle the issue of the Intel SGX SDK's Null-terminated string. The policy we enforced on Ocalls (P1) will make sure the arguments are valid.

Comment 3. *”...it is not clear what the advantage of the suggested approach over using type-safe languages or mechanisms such as suggested for Google Chrome Native Clients...”*

One important downside of a type-safe intermediate language (IL) is that no current formal tools can transform a binary to IL for verification inside Intel SGX enclave. 

And compared with a sandbox implementation for SGX (e.g., Ryoan at OSDI `16) that adds more TCB and computations, our work only consists of less than 2 MB binary code as the TCB and has much better performance than approaches using other mechanisms.

Comment 4. *”Side channel attacks are considered out-of-scope for the paper...”*

Side channels are difficult to eliminate since they are close related to the hardware architecture. Nevertheless, we illustrate that we can insert proof to mitigate the AEX-based side channel leakages.

Comment 5. *”...Can the verified code communicate with the service provider? Can it use longjmp? Is multithreading supported? etc.”*

Setjmp/longjmp is disallowed in our system since they can break
call-return semantics. Multi-threading/Multi-user is supported. Other discussions are made in Section~\ref{sec-discussion}.

To Review B:

Comment 1. *“The lack of covert channel protection is very problematic ..."*

We added new policies on side channel/covert channel prevention.

Comment 2. *”The only supported policy is that no data is written outside the enclave...”*

Besides the policy that no data is written outside the enclave, the CAT-SGX system now supports categories of security policies, including data leak control, control-transfer management, self-modifying code block and side/covert channel mitigation (Section~\ref{subsec-policies}).

Comment 3. *”The paper is riddled with typos.”*

Mentioned typos are carefully rectified.

Comment 4. *”This isn't proof-carrying code.  It's instrumented code.”*

According to XFI (OSDI `06) (a paper coauthored by George C. Necula, the designer of PCC) XFI modules can be seen as an example of proof-carrying code, even though they do not include logical proofs. Similar as XFI our work uses static analysis with inline software guards that perform checks at runtime, which could be regarded as an example of PCC that trusts only the verifier, not the means of proof generation.

Comment 5. *”I'm not clear why this would be better in practice than a LISP interpreter with some security/privacy policy annotations.”*

First of all, an enclave program is designed written in C/C++
Comparing to formal verification, generating security annotations is significantly less weighted, allowing our solution to scale to real world software

Comment 6. *”...why must the loader be in the same enclave as the running code?  Surely verifying it from afar would be safer and would avoid some of this CFI mess?”*

CFI is still needed even two enclaves are applied. 
CFI is a meaningful confidentiality policy because it guarantees that attackers cannot hijack the control flow and bypass the check, even when the attack collude with the service code provider.
The only advantage of using two enclave is that there will be No W+X issue during the binary loading, which in return can be dealt with the software DEP. However, using two enclave may induce more communication overhead 
%And the attestation protocol should be re-designed, while introduces larger TCB and more overhead since more parties are involved.
and we still need a binary rewriter within the bootstrap enclave. We believe both designs are reasonable. However, at this time, we may stick to the original `one-enclave' design for the following reasons: memory store operation instrumentation can be easily extended to support W+X. With the one-enclave design, the code of resolving symbols (during loading) can be easily reused by the rewritter and the verifier which reduces the memory consumption of SGX memory. 
%One-enclave design is more compact and cute, which leads a smaller TCB.

To Review C:

Comment 1. *“The CAT model has been proposed and studied extensively...- private data objects (Intel): https://arxiv.org/abs/1807.05686
- similar paper (cheng et al): https://arxiv.org/abs/1804.05141
and others."*

Those two papers only care about the data privacy, but not the smart contract's secrecy. Thus, the CAT model is not exactly the same with them.

Comment 2. *“...Bolting on DEP etc protections to cover for SGX v1 details seems unnecessary -- can this be skipped?"*

The goal of enforcing DEP was elaborated (since the bootstrap enclave built on SGXv1 ....)

The DEP can not be skipped since the loaded binary will be allocated on enclave's heap memory, leading to a W+X problem.

Comment 3. *“Should these be enforced in hardware (if the goal is to use hardware-based enclaves like SGX)? Why should this require a proof-carrying code..."*

Although Intel SGX provides good security guarantees, an enclave still can write data outside of its EPC memory region arbitrarily. Thus, we need to make various ground rules which are not naturally supported in SGX to screen and prevent such memory operations and the integrity of the check itself.

Allocating the tasks across untrusted and trusted parts unbalanced, with one generating the proof while a simpler trusted part checks it inside the enclave, will result in a very small TCB and computation on the trusted parts. As a PCC example, CAT-SGX can make sure the properties are checked only by verifying if the proof exists.

Comment 4. *“I can see why one might want to verify side-channel security of code that runs inside an enclave and ensuring that side-channel defenses compiled into the code indeed check off certain properties.*“

We added policies and demonstrated that side channels can be checked through proof compiled into the code. 

}
